# Supplementary material for: Deep Prior Learning for Embodied Perception
Source: arXiv:2610.05531 source file (2026-10-04)
Supplement: Supplementary file 2 [file appendix_trained_tables.tex]

\clearpage
\subsubsection{TartanAir-V2}
\input{tables/generated/trained_v2_pose.tex}
\input{tables/generated/trained_v2_directed.tex}
\input{tables/generated/trained_v2_depth.tex}
\input{tables/generated/trained_v2_retention.tex}
\clearpage
\subsubsection{Virtual KITTI 2}
\input{tables/generated/trained_vkitti-eval_pose.tex}
\input{tables/generated/trained_vkitti-eval_directed.tex}
\input{tables/generated/trained_vkitti-eval_depth.tex}
\input{tables/generated/trained_vkitti-eval_retention.tex}
\clearpage
\subsubsection{TUM RGB-D}
\input{tables/generated/trained_tum-eval_pose.tex}
\input{tables/generated/trained_tum-eval_directed.tex}
\input{tables/generated/trained_tum-eval_depth.tex}
\input{tables/generated/trained_tum-eval_retention.tex}
\clearpage
\subsubsection{C3VD}
\input{tables/generated/trained_c3vd-eval_pose.tex}
\input{tables/generated/trained_c3vd-eval_directed.tex}
\input{tables/generated/trained_c3vd-eval_depth.tex}
\input{tables/generated/trained_c3vd-eval_retention.tex}
